# Supplementary material for: Deep generative models as an adversarial attack strategy for tabular machine learning
Source: arXiv:2409.12642 source file (2024-09-19)
Supplement: Supplementary file 1 [file advCDGM.tex]

\newpage
\newpage
\clearpage
\section{Realism of adversarial examples from Deep
Generative Models}

\subsection{Appendix A: Context on collaboration for Chapter \ref{chap:advCDGM}}
\label{app:collaboration}
To utilize DGMs as an adversarial method for testing the robustness of ML models, while ensuring compliance with background knowledge, we devised a two-step approach:

\begin{itemize}
\item Expand DGMs to C-DGMs through a differentiable layer capable of repairing constraints.

\item Transform tabular C-DGMs into adversarial generation techniques C-AdvDGMs by performing functional modifications.
\end{itemize}
However, the first step would require some expertise in Neuro-symbolic AI, which we do not possess. Therefore, we collaborated with researchers from University of Oxford and Vienna University of Technology who have previously worked in this area. Our joint efforts resulted in the publication of our findings as a conference paper \cite{SDCLG-ICLR-2024}. Some of the results of this work are presented in Section \ref{subsec:exp_violations}, \ref{sec:exp_quality} and Appendix \ref{app:iclr_results}. The individual contributions to obtain those results are as below: 

\begin{itemize}
    \item Design and implementation of the constrained layer CL (Mihaela Stoian). 
    \item Running experiments for WGAN and GOGGLE models (Mihaela Stoian), for CTGAN, TVAE (Salijona Dyrmishi), for TableGAN (Mihaela Stoian and Salijona Dyrmishi)
    \item Converting data transforms into differentiable operations for CTGAN \& TVAE (Salijona Dyrmishi)
\end{itemize}

\subsection{Appendix B: Experimental analysis settings}\label{app:exp_settings}

\subsubsection{Models}
\label{app:models}
In our experimental analysis, we use five base models:

\begin{itemize}

    \item \textbf{WGAN}~\cite{Arjovsky2017_WGAN} is a GAN model trained with Wasserstein loss in a typical generator discriminator GAN-based architecture. In our implementation, WGAN uses a MinMax transformer for the continuous features and one-hot encoding for categorical ones. It has not been designed specifically for tabular data. 

    \item \textbf{TableGAN}~\cite{park2018_tableGAN} is among the first GAN-based approaches proposed for tabular data generation. In addition to the typical generator and discriminator architecture for GANs, the authors proposed adding a classifier trained to learn the relationship between the labels and the other features. The classifier ensures a higher number of semantically correct produced records. TableGAN uses a MinMax transformer for the features. 
    
    \item \textbf{CTGAN}~\cite{xu2019_CTGAN} uses a  conditional generator and training-by-sampling strategy in a generator-discriminator GAN architecture to model tabular data.  The conditional generator generates synthetic rows conditioned on one of the discrete columns. The training-by-sampling ensures that the data are sampled according to the log-frequency of each category. Both help to better model the imbalanced categorical columns. CTGAN transforms discrete features using one-hot encoding and a mode-based normalization for continuous features. A variational Gaussian mixture model~\cite{camino2018_vgm} is used to estimate the number of modes and fit a Gaussian mixture. For each continuous value, a mode is sampled based on probability densities, and its mean and standard deviation are used to normalize the value. 

    \item \textbf{TVAE} \cite{xu2019_CTGAN} was proposed as a variation of the standard Variational AutoEncoder to handle tabular data. It uses the same transformations of data as CTGAN and trains the encoder-decoder architecture using evidence lower-bound 
 (ELBO) loss.

    \item \textbf{GOGGLE}\cite{liu2022goggle} is a graph-based approach to learning the relational structure of the data as well as functional relationships (dependencies between features). The relational structure of the data is learned by building a graph where nodes are variables and edges indicate dependencies between them. The functional dependencies are learned through a message passing neural network (MPNN). The generative model generates each variable considering its surrounding neighborhood.
    % \item \textbf{OCTGAN} \cite{kim2021oct} is another variant of CTGAN where the generator and discriminator architecture are based on neural ordinary differential equations (NODEs).
    
\end{itemize}

\subsubsection{Datasets}
\label{app:datasets}

We use 5 real-world datasets, and an overview of these datasets' statistics can be found in Table~\ref{tab:app_dataset}. 
For the selection, we focused on datasets with at least three feature relationship constraints that either were provided with the description of the datasets or we could derive with our domain expertise. The selected datasets are listed below: 

\begin{itemize}
    \item \phishing\footnote{Link to dataset: https://data.mendeley.com/datasets/c2gw7fy2j4/2}~\cite{hannousse2021towards} is used to perform webpage phishing detection with features describing statistical properties of the URL itself as well as the content of the page. 
    \item \wids\footnote{Link to dataset: https://www.kaggle.com/competitions/widsdatathon2021} is used to predict if a patient is diagnosed with a particular type of diabetes named Diabetes Mellitus, using data from the first 24 hours of intensive care. 
    \item \lcld{}\footnote{Link to dataset: https://figshare.com/s/84ae808ce6999fafd192} is used to predict whether the debt lent is unlikely to be collected. In particular, we use the feature-engineered dataset from~\cite{simonetto2022}, inspired from the LendingClub loan data. The dataset captures features related to the loan as well as client history.
    % \item  \botnet \cite{chernikova2022fence} is used to predict botnet traffic using aggregated network data.  
    \item FICO's Home Equity Line of Credit dataset (\heloc{}\footnote{Link to the dataset: https://huggingface.co/datasets/mstz/heloc}) from the FICO xML Challenge is used to predict whether customers will repay their credit lines within 2 years. Similarly to \lcld, the dataset has features related to the credit line and the client's history. 
    \item \faults{}\footnote{Link to dataset: https://www.kaggle.com/datasets/uciml/faulty-steel-plates}\cite{buscema1998metanet} is used to predict 7 types of surface defects in stainless steel plates. The features approximately capture the geometric shape of the defect and its outline. 
\end{itemize}

For \phishing{}, \wids{}, and \lcld{}, we used the train-val-test splits provided by \cite{simonetto2022}. 
For \heloc{} we used the train-test split of 80-20 and 20\% of the training set was later split for validation. 
Finally, for \faults{} and \news{} we split the data into 80-10-10\% sets, and for the former (which is a multiclass classification dataset) we preserved the class imbalance.

\begin{table}[ht!]
\centering
\caption{Datasets statistics.}
\begin{tabular}{@{}lccccccc@{}}
\toprule
\multicolumn{1}{c}{Dataset} & \# Train & \# Val & \# Test & \# Feat. & \# Cat. & \# Cont. & \# C. \\ \midrule
\phishing & 7K       & 2K     & 2K      & 64          & 20      & 44       & 2         \\
\wids     & 22K      & 6K     & 7K      & 109         & 9       & 100      & 2         \\
\lcld     & 494K     & 199K   & 431K    & 29          & 8       & 21       & 2         \\
\heloc    & 8K       & 2K     & 0.2K    & 24          & 8       & 16       & 2         \\
\faults   & 2K       & 0.2K   & 0.2K    & 28          & 0       & 28       & 7         \\ \bottomrule
\end{tabular}
\label{tab:app_dataset}
\end{table}

\subsubsection{Constraints Datasheet}
\label{app:constraints}

Here, we outline the structure of our constraints. Let \( F \) denote the number of features that appear in at least one constraint, while \( D \) represents the total number of features. For any given constraint \(\phi\), we define \( F^+_{\phi} \) as the number of features appearing positively in \(\phi\), and \( F^-_{\phi} \) as the number of features appearing negatively. The total number of features appearing in \(\phi\) is \( F_{\phi} = F^+_{\phi} + F^-_{\phi} \).

As illustrated in Table~\ref{tab:app_cons}, the characteristics of constraints vary significantly across different datasets. The number of constraints annotated per dataset ranges from 4 to 31. The percentage of variables appearing in at least one constraint varies from as low as 17.2\% in \lcld{} to as high as 56.88\% in \wids{}. Additionally, for almost all datasets, the average number of features per constraint is 2.00. However, \phishing{} stands out with one constraint involving 17 different features, and \lcld{} has two constraints where only a single variable appears. %Finally, as we can see in the last column, in each dataset, if a feature

\begin{table}[ht!]
    \centering
    \caption{Constraints statistics.}
    \begin{tabular}{l r r r r r r r r}
    \toprule
        Dataset &  \# Constr. & $F$ / $D$   & Avg. $F_\phi$ & Avg. $F_{\phi}^+$  & Avg. $F_{\phi}^-$ \\ % Avg. $C_i$ \\
        \midrule
         \phishing{} & 8 &  24 / 64 \ &  4.25 & 1.00 & 3.25 \\ % & 1.42 \\
         \wids{} & 31 & 62 / 109 &2.00 & 1.00 & 1.00 \\ % & 1.00   \\
         \lcld{} & 4 & \ 5 / 29 \    &1.50 & 0.75 & 0.75 \\ % & 1.20    \\
         % \botnet{} & 366 & 468/757 & 3.92 & 1.96 & 1.96 & 3.07 & 288 & 3.85 \\
         \heloc{} & 7 & 10 / 24 \  &2.00 & 1.00 & 1.00 \\ % & 1.40   \\
         \faults{} & 4 & \  7 / 28 \  &2.00 & 1.00 & 1.00 \\ % & 1.14    \\
      \bottomrule   
    \end{tabular}
    \label{tab:app_cons}
\end{table}

\subsubsection{Evaluation protocol for C-DGMs}
\label{app:eval_protocol}

For evaluating the utility of the DGM/C-DGM models presented in our paper, we followed closely the protocol from \cite{kim2023stasy} which we also reproduce here.
\begin{enumerate}
    \item First, we generate a synthetic dataset, split into training, validation and test partitions using the same proportions as the real dataset.
    \item Then, we perform a hyperparameter search using the synthetic training data partition to train different classifiers/regressors.
    % \item Lastly, we use the best set of hyperparameters for each classifier/regressor to train and test our models in synthetic data.
    
For the binary classification datasets (i.e., \phishing{}, \wids{}, \lcld{}, and \heloc{}) we use: Decision Tree~\cite{decision_tree}, AdaBoost~\cite{adaboost},  Multi-layer Perceptron (MLP)~\cite{MLP}, Random Forest~\cite{random_forest}, XGBoost~\cite{xgboost}, and Logistic Regression~\cite{logistic_regression} classifiers.
For multi-class classification datasets, (i.e., \faults{}) we use Decision Tree, MLP, Random Forest, and XGBoost classifiers.
For the regression dataset, (i.e., \news{}) we use MLP, XGBoost, and Random Forest regressors and linear regression.
For all the classifiers and regressors above, we considered the same hyperparameter settings as those from Table 26 of~\cite{kim2023stasy} and picked the best hyperparameter configuration using the real validation set according to the F1-score. 

% TODO: double check it's f1 score and not average over f1s and aucroc when picking best model/ talk about metrics, f1, wf1, aucroc used for picking best model.

    \item Finally, we tested the selected best models on the real test set and averaged the results across all the classifiers/regressors to get performance measurements for the DGM/C-DGM predictions according to three different metrics: F1-score, weighted F1-score, and Area Under the ROC Curve.
\end{enumerate}

The above procedure was repeated 5 times for each DGM/C-DGM model, and the results were averaged separately for each of the metrics.

For evaluating the DGM/C-DGM models in terms of detection, we slightly adapted the procedure presented by \cite{kim2023stasy}.
We first created the training, validation, and test sets by concatenating real and synthetic data, including their targets as usual features, and adding a new target column that specifies whether the data is real or not.
By construction, these datasets are binary classification datasets and, thus, are suitable for the hyperparameter search procedure presented in \cite{kim2023stasy} using the 6 different binary classifiers mentioned above.
We proceeded to pick the best model using the newly-created validation set, and then we obtained the final detection performance on the newly-created test data (which combines the real and the synthetic data).

\subsection{Appendix C: Results}
\label{app:iclr_results}

\subsubsection{Effect on boundary population by CL}
To investigate the properties of data generated by C-DGMs, we examine the impact of constraint reparation on the boundary population for the WiDS, HELOC, and FSP datasets, which had the most violated constraints. We defined a band around the boundary with a width \( w \), proportional to the range of the feature values in the real dataset. Since all the considered constraints involve only two features, we set \( w = \sqrt{(r_1p)^2 + (r_2p)^2} \), where \( r_1 \) and \( r_2 \) represent the range of the first and second features respectively, and \( p \) represents the proportion of the range of values each feature can take. If \( p = 1 \), the width equals the diagonal of the rectangle defined by the minimum and maximum coordinates.

Table \ref{tab:border metrics} shows the percentage of generated samples that lie on the boundary for \( p = \{1\%, 5\%, 10\%\} \) for the real dataset (last row), individual DGMs, and C-DGMs, as well as their averages (third and second to last rows, respectively). The results indicate that C-DGMs populate the boundary at a rate much closer to the real data than their unconstrained counterparts. Specifically, the maximum difference between the percentage of real data points on the boundary and the average number of samples generated by C-DGMs is 14.7\% (for the WiDS dataset and \( p = 1\% \)). In contrast, the maximum difference for DGMs is 51.5\% (for the Faults dataset and \( p = 1\% \)).
\begin{table}[ht!]
\centering
\small
\caption{Percentage of the generated samples that lie on the boundary.}
\setlength{\tabcolsep}{2pt}
\label{tab:border metrics}
\begin{tabular}{@{}llll@{\hspace{15pt}}lll@{\hspace{15pt}}lll}
\toprule
           & \multicolumn{3}{c}{\wids}             & \multicolumn{3}{c}{\heloc}               & \multicolumn{3}{c}{\faults}           \\ \cmidrule(lr){2-4} \cmidrule(l){5-7} \cmidrule(l){8-10} 
          $p$ & $1\%$       & $5\%$       & $10\%$      & $1\%$       & $5\%$        & $10\%$       & $1\%$       & $5\%$       & $10\%$      \\ \cmidrule(r){1-2}

WGAN       & 28.5   & 45.2   & 67.0   & 22.5   & 83.9   & 99.4   & 14.8   & 55.6   & 81.2  \\
C-WGAN     & 62.1   & 72.1   & 83.1   & 100.0  & 100.0  & 100.0  & 76.8   & 83.1   & 89.9  \\ \cmidrule(lr){1-1}
TableGAN   & 19.7   & 71.9   & 88.7   & 37.4   & 94.7   & 99.8   & 25.3   & 76.0   & 95.8  \\
C-TableGAN & 72.2   & 81.1   & 88.7   & 83.8   & 96.1   & 99.1   & 75.4   & 86.2   & 94.3  \\ \cmidrule(r){1-1}
CTGAN      & 6.5    & 30.5   & 53.2   & 80.2   & 93.1   & 96.8   & 2.6    & 16.4   & 36.7  \\
C-CTGAN    & 54.2   & 62.4   & 73.8   & 83.2   & 96.0   & 98.3   & 49.2   & 62.3   & 72.9  \\ \cmidrule(r){1-1}
TVAE       & 20.2   & 42.0   & 62.4   & 69.4   & 90.1   & 96.5   & 6.5    & 37.6   & 56.7  \\
C-TVAE     & 31.0   & 56.9   & 69.7   & 79.2   & 92.7   & 97.1   & 38.4   & 57.5   & 77.4  \\ \cmidrule(r){1-1}
GOGGLE     & 0.9    & 29.1   & 33.1   & 46.3   & 99.6   & 100.0  & 35.3   & 82.2   & 98.9  \\
C-GOGGLE   & 7.7    & 77.2   & 99.1   & 83.9   & 92.4   & 97.0   & 81.1   & 85.4   & 89.7  \\ \cmidrule(r){1-1}
DGMs       & 15.2   & 43.8   & 60.9   & 51.1   & 92.3   & 98.5   & 16.9   & 53.5   & 73.9  \\
C-DGMs     & 45.4   & 69.9   & 82.9   & 86.0   & 95.4   & 98.3   & 64.2   & 74.9   & 84.8  \\ \cmidrule(r){1-1}
Real       & 60.1   & 73.3   & 85.1   & 85.7   & 96.5   & 98.9   & 68.4   & 82.8   & 98.9  \\
\bottomrule
\end{tabular}
\end{table}

\subsubsection{Full results on DGMs vs. P-DGMs vs C-DGMs}
\label{appendix:full_cdgm}

In this section, we present the individual results for each datasets for all the models under study. Respectively for WGAN in Table \ref{appendix:wgan_full}, for TableGAN in \ref{appendix:tablegan_full}, for CTGAN in \ref{appendix:ctgan_full}, for TVAE in \ref{appendix:tvae_full} and for GOGGLE in \ref{appendix:goggle_full}

\begin{table}[ht!]
\caption{Utility and detection results for individual datasets for WGAN.}
\label{appendix:wgan_full}
\centering
\begin{tabular}{ll ccc ccc}
 \toprule
    &   & \multicolumn{3}{c}{\bf{Utility} ($\uparrow$)} & \multicolumn{3}{c}{\bf{Detection} ($\downarrow$)} \\
        \cmidrule(lr){3-5} \cmidrule(lr){6-8}
       &  & F1 & {\sl w}F1 & AUC & F1 & {\sl w}F1 & AUC \\
\cmidrule(r){1-2}
URL & WGAN & 0.756 & 0.764 & 0.839 & 0.865 & 0.856 & 0.872 \\
 & P-WGAN & 0.767 & 0.768 & 0.840 & 0.856 & 0.852 & 0.867 \\
 & C-WGAN & \textbf{0.792} & \textbf{0.782} & \textbf{0.860} & \textbf{0.864} & \textbf{0.851} & \textbf{0.877} \\
\cmidrule(r){1-2}
Wids & WGAN & 0.329 & 0.381 & 0.775 & 0.975 & 0.976 & 0.989 \\
 & P-WGAN & 0.334 & 0.386 & 0.783 & 0.978 & 0.978 & 0.991 \\
 & C-WGAN & \textbf{0.316} & \textbf{0.373} & \textbf{0.816} & \textbf{0.975} & \textbf{0.975} & \textbf{0.989} \\
\cmidrule(r){1-2}
LCLD & WGAN & \textbf{0.239} & \textbf{0.359} & \textbf{0.618} & \textbf{0.999} & \textbf{0.999} & \textbf{1.000} \\
 & P-WGAN & 0.214 & 0.352 & 0.617 & 0.921 & 0.914 & 0.942 \\
 & C-WGAN & 0.232 & 0.358 & 0.612 & 0.923 & 0.917 & 0.946 \\
\cmidrule(r){1-2}
HELOC & WGAN & 0.634 & 0.599 & 0.677 & 0.964 & 0.964 & 0.983 \\
 & P-WGAN & \textbf{0.641} & 0.600 & 0.682 & 0.964 & 0.965 & \textbf{0.985} \\
 & C-WGAN & \textbf{0.711} & \textbf{0.649} & \textbf{0.715} & \textbf{0.957} & \textbf{0.957} & 0.975 \\
\cmidrule(r){1-2}
Faults & WGAN & 0.357 & 0.339 & 0.742 & 0.914 & 0.910 & 0.916 \\
 & P-WGAN & 0.355 & 0.337 & 0.736 & 0.910 & 0.907 & 0.927 \\
 & C-WGAN & \textbf{0.367} & \textbf{0.349} & \textbf{0.742} & \textbf{0.843} & \textbf{0.845} & \textbf{0.874} \\
\bottomrule
\end{tabular}
\end{table}

\begin{table}[ht!]
\caption{Utility and detection results for individual datasets for TableGAN.}
\label{appendix:tablegan_full}
\centering
\begin{tabular}{ll ccc ccc}
 \toprule
    &   & \multicolumn{3}{c}{\bf{Utility} ($\uparrow$)} & \multicolumn{3}{c}{\bf{Detection} ($\downarrow$)} \\
        \cmidrule(lr){3-5} \cmidrule(lr){6-8}
       &  & F1 & {\sl w}F1 & AUC & F1 & {\sl w}F1 & AUC \\
\cmidrule(r){1-2}
URL & TableGAN & 0.562 & 0.659 & 0.843 & 0.831 & 0.822 & 0.850 \\
 & P-TableGAN & 0.565 & 0.660 & 0.848 & 0.843 & 0.823 & 0.850 \\
 & C-TableGAN & \textbf{0.611} & \textbf{0.695} & \textbf{0.868} & \textbf{0.849} & \textbf{0.835} & \textbf{0.856} \\
\cmidrule(r){1-2}
Wids & TableGAN & 0.171 & 0.240 & 0.740 & 0.963 & 0.964 & 0.980 \\
 & P-TableGAN & 0.173 & 0.243 & 0.749 & 0.962 & 0.963 & 0.980 \\
 & C-TableGAN & \textbf{0.246} & \textbf{0.309} & \textbf{0.775} & \textbf{0.956} & \textbf{0.957} & \textbf{0.974} \\
\cmidrule(r){1-2}
LCLD & TableGAN & \textbf{0.123} & \textbf{0.286} & \textbf{0.587} & \textbf{0.895} & \textbf{0.895} & \textbf{0.926} \\
 & P-TableGAN & 0.115 & 0.281 & 0.585 & 0.896 & 0.888 & 0.925 \\
 & C-TableGAN & 0.174 & 0.314 & 0.587 & 0.869 & 0.871 & 0.909 \\
\cmidrule(r){1-2}
HELOC & TableGAN & 0.593 & 0.615 & 0.707 & 0.923 & 0.925 & 0.953 \\
 & P-TableGAN & 0.594 & 0.614 & 0.707 & 0.922 & 0.924 & 0.953 \\
 & C-TableGAN & \textbf{0.638} & \textbf{0.633} & \textbf{0.705} & \textbf{0.952} & \textbf{0.952} & \textbf{0.970} \\
\cmidrule(r){1-2}
Faults & TableGAN & 0.199 & 0.199 & 0.642 & 0.909 & 0.906 & 0.907 \\
 & P-TableGAN & 0.194 & 0.195 & 0.645 & 0.860 & 0.868 & 0.886 \\
 & C-TableGAN & \textbf{0.208} & \textbf{0.209} & \textbf{0.635} & \textbf{0.830} & \textbf{0.817} & \textbf{0.849} \\
\bottomrule
\end{tabular}
\end{table}

\begin{table}[ht!]
\caption{Utility and detection results for individual datasets for CTGAN.}
\label{appendix:ctgan_full}
\centering
\begin{tabular}{ll ccc ccc ccc}
    \toprule
    &   & \multicolumn{3}{c}{\bf{Utility} ($\uparrow$)} & \multicolumn{3}{c}{\bf{Detection} ($\downarrow$)} \\
        \cmidrule(lr){3-5} \cmidrule(lr){6-8}
       &  & F1 & {\sl w}F1 & AUC & F1 & {\sl w}F1 & AUC \\
\cmidrule(r){1-2}
URL & CTGAN & 0.822 & 0.799 & 0.859 & 0.850 & 0.862 & 0.879 \\
 & P-CTGAN & 0.823 & 0.802 & 0.863 & 0.850 & 0.861 & 0.876 \\
 & C-CTGAN & \textbf{0.830} & \textbf{0.816} & \textbf{0.877} & \textbf{0.820} & \textbf{0.839} & \textbf{0.864} \\
\cmidrule(r){1-2}
Wids & CTGAN & 0.362 & 0.405 & 0.835 & 0.990 & 0.990 & 0.996 \\
 & P-CTGAN & 0.365 & 0.407 & 0.835 & \textbf{0.989} & \textbf{0.989} & \textbf{0.997} \\
 & C-CTGAN & \textbf{0.365} & \textbf{0.408} & \textbf{0.837} & 0.990 & 0.990 & 0.997 \\
\cmidrule(r){1-2}
LCLD & CTGAN & \textbf{0.290} & \textbf{0.407} & \textbf{0.657} & 0.836 & 0.847 & \textbf{0.889} \\
 & P-CTGAN & 0.255 & 0.383 & 0.652 & 0.839 & 0.840 & 0.892 \\
 & C-CTGAN & 0.265 & 0.392 & 0.641 & \textbf{0.848} & \textbf{0.837} & 0.897 \\
\cmidrule(r){1-2}
HELOC & CTGAN & 0.736 & 0.675 & 0.744 & 0.914 & 0.915 & \textbf{0.953} \\
 & P-CTGAN & \textbf{0.743} & 0.678 & 0.745 & \textbf{0.913} & \textbf{0.914} & 0.952 \\
 & C-CTGAN & 0.736 & \textbf{0.690} & \textbf{0.751} & 0.897 & 0.897 & 0.943 \\
\cmidrule(r){1-2}
Faults & CTGAN & 0.374 & 0.372 & \textbf{0.760} & 0.926 & 0.927 & \textbf{0.932} \\
 & P-CTGAN & 0.372 & 0.370 & 0.754 & 0.895 & 0.902 & 0.922 \\
 & C-CTGAN & \textbf{0.381} & \textbf{0.380} & 0.759 & \textbf{0.857} & \textbf{0.868} & 0.893 \\
\bottomrule
\end{tabular}
\end{table}

% Please add the following required packages to your document preamble:
% \usepackage{booktabs}
\begin{table}[ht!]
\centering
\caption{Utility and detection results for individual datasets for TVAE.}
\label{appendix:tvae_full}
\begin{tabular}{ll ccc ccc ccc}
    \toprule
    &   & \multicolumn{3}{c}{\bf{Utility} ($\uparrow$)} & \multicolumn{3}{c}{\bf{Detection} ($\downarrow$)} \\
        \cmidrule(lr){3-5} \cmidrule(lr){6-8}
       &  & F1 & {\sl w}F1 & AUC & F1 & {\sl w}F1 & AUC \\
\cmidrule(r){1-2}
URL    & TVAE    & 0.810     & 0.802       & 0.863   & 0.813     & 0.831       & 0.854   \\
       & P-TVAE  & 0.815     & 0.806       & 0.870   & \textbf{0.806}     & \textbf{0.829}       & \textbf{0.850}   \\
       & C-TVAE  & \textbf{0.824}     & \textbf{0.816}       & \textbf{0.879}   & 0.814     & 0.829       & 0.849   \\ \cmidrule(r){1-2}
Wids   & TVAE    & 0.282     & 0.342       & 0.800   & \textbf{0.926}     & \textbf{0.927}       & \textbf{0.935}   \\
       & P-TVAE  & 0.285     & 0.344       & 0.797   & 0.964     & 0.964       & 0.979   \\
       & C-TVAE  & \textbf{0.322}     & \textbf{0.378}       & \textbf{0.815}   & 0.961     & 0.962       & 0.979   \\ \cmidrule(r){1-2}
LCLD   & TVAE    & \textbf{0.185}     & \textbf{0.330}       & \textbf{0.631}   & \textbf{0.842}     & \textbf{0.832}       & \textbf{0.861}   \\
       & P-TVAE  & 0.176     & 0.325       & 0.629   & 0.829     & 0.825       & 0.858   \\
       & C-TVAE  & 0.158     & 0.311       & 0.633   & 0.808     & 0.795       & 0.840   \\ \cmidrule(r){1-2}
HELOC  & TVAE    & \textbf{0.735}     & \textbf{0.696}       & \textbf{0.752}   & \textbf{0.914}     & \textbf{0.916}       & \textbf{0.947}   \\
       & P-TVAE  & \textbf{0.735}     & 0.694       & 0.750   & 0.909     & 0.910       & 0.944   \\
       & C-TVAE  & 0.733     & 0.690       & 0.749   & 0.905     & 0.908       & 0.943   \\ \cmidrule(r){1-2}
Faults & TVAE    & 0.473     & 0.463       & 0.789   & \textbf{0.843}     & \textbf{0.847}       & \textbf{0.872}   \\
       & P-TVAE  & 0.463     & 0.453       & 0.788   & 0.874     & 0.870       & 0.895   \\
       & C-TVAE  & \textbf{0.496}     & \textbf{0.488}       & \textbf{0.791}   & 0.855     & 0.857       & 0.896   \\ \bottomrule
\end{tabular}
\end{table} 
% Please add the following required packages to your document preamble:
% \usepackage{booktabs}

\begin{table}[ht!]
\centering
\caption{Utility and detection results for individual datasets for GOGGLE.}
\label{appendix:goggle_full}
\begin{tabular}{ll ccc ccc}
    \toprule
    &   & \multicolumn{3}{c}{\bf{Utility} ($\uparrow$)} & \multicolumn{3}{c}{\bf{Detection} ($\downarrow$)} \\
        \cmidrule(lr){3-5} \cmidrule(lr){6-8}
       &  & F1 & {\sl w}F1 & AUC & F1 & {\sl w}F1 & AUC \\
\cmidrule(r){1-2}
URL & GOGGLE & 0.622 & 0.648 & 0.742 & 0.892 & 0.880 & 0.891 \\
 & P-GOGGLE & 0.626 & 0.645 & 0.738 & 0.884 & 0.878 & 0.889 \\
 & C-GOGGLE & \textbf{0.782} & \textbf{0.741} & \textbf{0.800} & \textbf{0.890} & \textbf{0.891} & \textbf{0.898} \\
\cmidrule(r){1-2}
Wids & GOGGLE & 0.189 & 0.198 & 0.656 & 0.987 & 0.987 & 0.993 \\
 & P-GOGGLE & 0.193 & 0.202 & 0.665 & 0.988 & 0.988 & 0.994 \\
 & C-GOGGLE & \textbf{0.185} & \textbf{0.253} & \textbf{0.675} & \textbf{0.972} & \textbf{0.971} & \textbf{0.984} \\
\cmidrule(r){1-2}
LCLD & GOGGLE & \textbf{0.163} & \textbf{0.315} & \textbf{0.543} & 0.890 & 0.892 & \textbf{0.928} \\
 & P-GOGGLE & 0.164 & 0.315 & 0.548 & 0.892 & 0.889 & 0.923 \\
 & C-GOGGLE & 0.219 & 0.357 & 0.593 & \textbf{0.910} & \textbf{0.912} & 0.943 \\
\cmidrule(r){1-2}
HELOC & GOGGLE & 0.596 & 0.566 & 0.600 & 0.924 & 0.926 & \textbf{0.949} \\
 & P-GOGGLE & \textbf{0.601} & 0.566 & 0.601 & 0.926 & 0.927 & 0.952 \\
 & C-GOGGLE & \textbf{0.723} & \textbf{0.663} & \textbf{0.719} & \textbf{0.939} & \textbf{0.940} & 0.958 \\
\cmidrule(r){1-2}
Faults & GOGGLE & 0.152 & 0.139 & 0.577 & 0.912 & 0.916 & \textbf{0.920} \\
 & P-GOGGLE & 0.155 & 0.141 & 0.578 & 0.907 & 0.906 & 0.917 \\
 & C-GOGGLE & \textbf{0.136} & \textbf{0.121} & \textbf{0.546} & \textbf{0.884} & \textbf{0.817} & 0.865 \\
\bottomrule
\end{tabular}
\end{table}

\subsubsection{Real data performance for utility}
To ensure meaningful comparisons between our constrained DGM (C-DGM) models and the baseline unconstrained DGMs, we conducted a hyperparameter search. This process allowed us to closely approximate, and sometimes even surpass, the utility performance of real data. We present these results in Table \ref{tab:real-utility}, using the same evaluation metrics employed for measuring synthetic data utility performance: F1-score, weighted F1-score, and Area Under the ROC Curve. The evaluation followed the protocol outlined in Appendix \ref{app:eval_protocol}.

Compared to synthetic data, C-WGAN and C-CTGAN models showed utility scores similar to real data. Notably, C-TableGAN and C-TVAE approaches effectively closed the gap between synthetic and real data performance in several instances. For example, in the \lcld{} dataset, C-TableGAN matched or even slightly exceeded real data performance.
However, none of the DGM or C-DGM models approached real \faults{} data performance. The small size and multiclass nature of the datasets may pose challenges for DGM models in capturing patterns accurately.

\begin{table}[ht!]
\centering
%\vspace{-0.4cm}
\caption{Utility scores calculated on real data}
\label{tab:real-utility}
\begin{tabular}{@{}llll@{}}
\toprule
       & F1     & {\sl w}F1 & AUC\\ \midrule
\phishing{}    & 0.884$\spm$0.007  & 0.875$\spm$0.014 & 0.903$\spm$0.009\\
\wids{}   &     0.383$\spm$0.021          &    0.434$\spm$0.020           &        0.832$\spm$0.009  \\
\lcld{}   &     0.171$\spm$0.030  & 0.316$\spm$0.013 & 0.645$\spm$0.007 \\
\heloc{}  & 0.772$\spm$0.003 & 0.662$\spm$0.011 & 0.707$\spm$0.008  \\
\faults{} & 0.662$\spm$0.011 & 0.659$\spm$0.009 & 0.848$\spm$0.010  \\ \bottomrule
\end{tabular}
% \vspace{-1cm}
\end{table}

\textbf{AdvDGM attack performance}

\begin{table}[ht!]
\centering
\caption{Adversarial attack results for $\epsilon=0.3$}
\label{tab:eps0.3}
\begin{tabular}{lllll}
\hline
\textbf{Model} & \textbf{HELOC}       & \textbf{FSP}         & \textbf{URL}         & \textbf{WIDS}        \\ \hline
AdvWGAN        & \textbf{0.40$\pm$0.16} & 0.00$\pm$0.00          & 0.27$\pm$0.12          & 0.15$\pm$0.10          \\
P-AdvWGAN      & \textbf{0.40$\pm$0.16} & 0.00$\pm$0.00          & \textbf{0.75$\pm$0.10} & 0.34$\pm$0.06          \\
C-AdvWGAN      & 0.27$\pm$0.11          & \textbf{0.02$\pm$0.03} & 0.39$\pm$0.31          & \textbf{0.43$\pm$0.03} \\ \cline{1-1}
AdvTableGAN    & \textbf{0.05$\pm$0.04} & 0.00$\pm$0.00          & 0.15$\pm$0.04          & 0.06$\pm$0.03          \\
P-AdvTableGAN  & \textbf{0.05$\pm$0.04} & \textbf{0.04$\pm$0.02} & \textbf{0.28$\pm$0.02} & 0.17$\pm$0.06          \\
C-AdvTableGAN  & 0.03$\pm$0.01          & 0.02$\pm$0.01          & 0.04$\pm$0.09          & \textbf{0.25$\pm$0.02} \\ \cline{1-1}
AdvCTGAN       & 0.01$\pm$0.00          & 0.01$\pm$0.01          & 0.18$\pm$0.03          & 0.00$\pm$0.01          \\
P-AdvCTGAN     & 0.01$\pm$0.00          & \textbf{0.08$\pm$0.09} & \textbf{0.28$\pm$0.01} & 0.01$\pm$0.01          \\
C-AdvCTGAN     & \textbf{0.02$\pm$0.00} & 0.01$\pm$0.00          & 0.16$\pm$0.05          & \textbf{0.14$\pm$0.04} \\ \cline{1-1}
AdvTVAE        & 0.00$\pm$0.00          & 0.00$\pm$0.00          & 0.16$\pm$0.01          & 0.02$\pm$0.01          \\
P-AdvTVAE      & 0.00$\pm$0.00          & 0.00$\pm$0.00          & 0.28$\pm$0.02          & \textbf{0.08$\pm$0.01} \\
C-AdvTVAE      & \textbf{0.01$\pm$0.00} & 0.00$\pm$0.00          & \textbf{0.50$\pm$0.04} & 0.05$\pm$0.01          \\ \hline
\end{tabular}
\end{table}

\begin{table}[ht!]
\centering
\caption{Adversarial attack results for $\epsilon=0.4$}
\label{tab:eps0.4}
\begin{tabular}{lllll}
\hline
\textbf{Model} & \textbf{HELOC}           & \textbf{FSP}             & \textbf{URL}             & \textbf{WIDS}            \\ \hline
AdvWGAN        & \textbf{0.59 $\pm$ 0.14} & 0.02 $\pm$ 0.00          & 0.31 $\pm$ 0.15          & 0.25 $\pm$ 0.18          \\
P-AdvWGAN      & \textbf{0.59 $\pm$ 0.14} & \textbf{0.13 $\pm$ 0.01} & \textbf{0.89 $\pm$ 0.03} & 0.58 $\pm$ 0.02          \\
C-AdvWGAN      & 0.41 $\pm$ 0.14          & 0.11 $\pm$ 0.10          & 0.49 $\pm$ 0.34          & \textbf{0.66 $\pm$ 0.06} \\ \cline{1-1}
AdvTableGAN    & \textbf{0.09 $\pm$ 0.06} & 0.02 $\pm$ 0.00          & 0.15 $\pm$ 0.04          & 0.07 $\pm$ 0.03          \\
P-AdvTableGAN  & \textbf{0.09 $\pm$ 0.06} & \textbf{0.13 $\pm$ 0.01} & \textbf{0.28 $\pm$ 0.02} & \textbf{0.26 $\pm$ 0.02} \\
C-AdvTableGAN  & 0.06 $\pm$ 0.01          & 0.09 $\pm$ 0.02          & 0.06 $\pm$ 0.13          & \textbf{0.26 $\pm$ 0.02} \\ \cline{1-1}
AdvCTGAN       & 0.01 $\pm$ 0.00          & 0.01 $\pm$ 0.01          & 0.18 $\pm$ 0.03          & 0.01 $\pm$ 0.02          \\
P-AdvCTGAN     & 0.01 $\pm$ 0.00          & \textbf{0.16 $\pm$ 0.10} & 0.28 $\pm$ 0.01          & 0.03 $\pm$ 0.04          \\
C-AdvCTGAN     & \textbf{0.02 $\pm$ 0.00} & 0.08 $\pm$ 0.01          & \textbf{0.31 $\pm$ 0.06} & \textbf{0.24 $\pm$ 0.04} \\ \cline{1-1}
AdvTVAE        & 0.00 $\pm$ 0.00          & 0.00 $\pm$ 0.00          & 0.18 $\pm$ 0.01          & 0.05 $\pm$ 0.02          \\
P-AdvTVAE      & 0.00 $\pm$ 0.00          & \textbf{0.03 $\pm$ 0.00} & 0.31 $\pm$ 0.02          & \textbf{0.18 $\pm$ 0.01} \\
C-AdvTVAE      & \textbf{0.01 $\pm$ 0.00} & \textbf{0.03 $\pm$ 0.00} & \textbf{0.62 $\pm$ 0.04} & 0.15 $\pm$ 0.01          \\ \hline
\end{tabular}
\end{table}
